# Supplementary material for: Multipar-T: Multiparty-Transformer for Capturing Contingent Behaviors in Group Conversations
Source: arXiv:2304.12204 source file (2023-04-19)
Supplement: Supplementary file 1 [file 99_appendix.tex]

\newpage

\onecolumn

\section{Additional Qualitative Examples}
\label{aref:qual}
\begin{figure*}[!ht]
    \centering
    \includegraphics[width=0.5\textwidth]{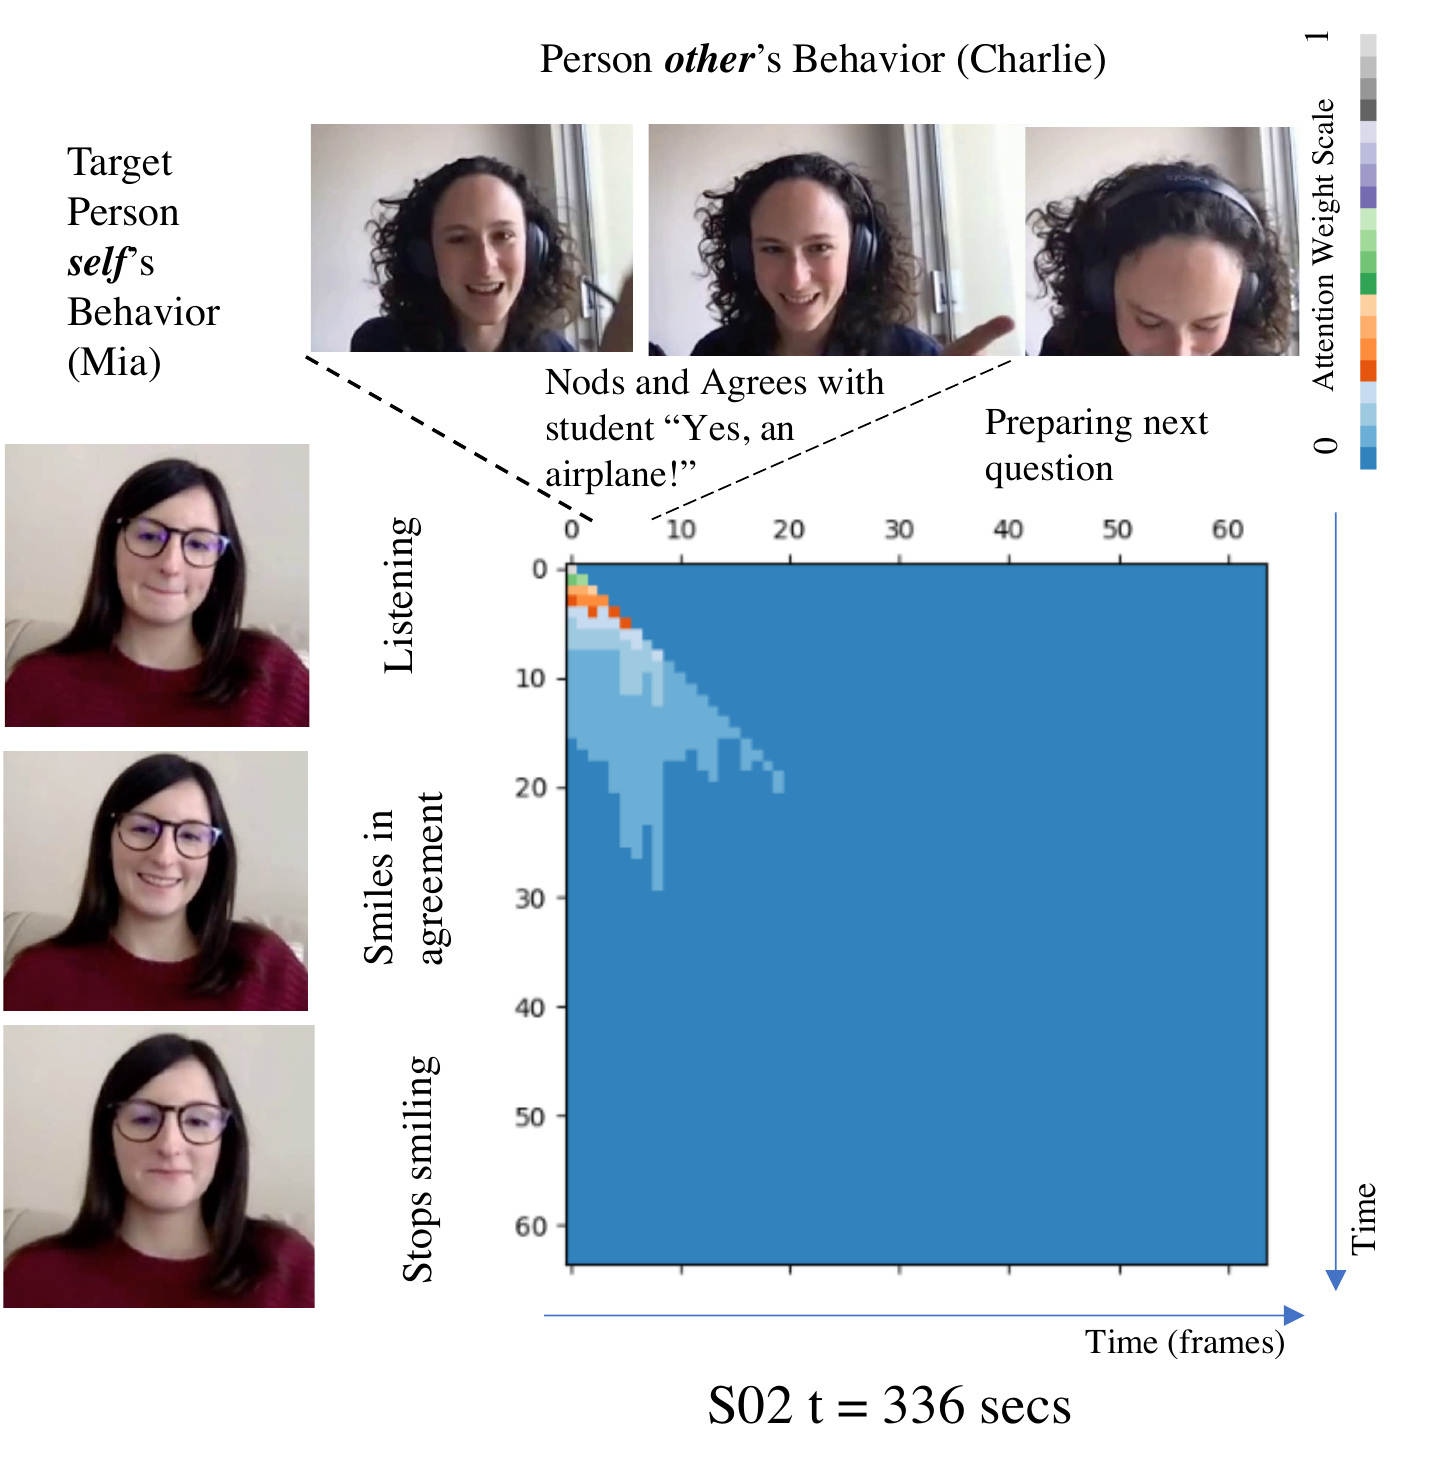}
    \caption{(a) \modelss Cross-person Attention weights from $t=336s$ for group $S02$. \modelshorts has discovered that $self$’s behavior from timestep 4-10 is contingent on $other$’s behavior in timestep 10 – 35 (smile). }

\end{figure*}

\begin{figure*}[!ht]
    \centering
    \includegraphics[width=0.5\textwidth]{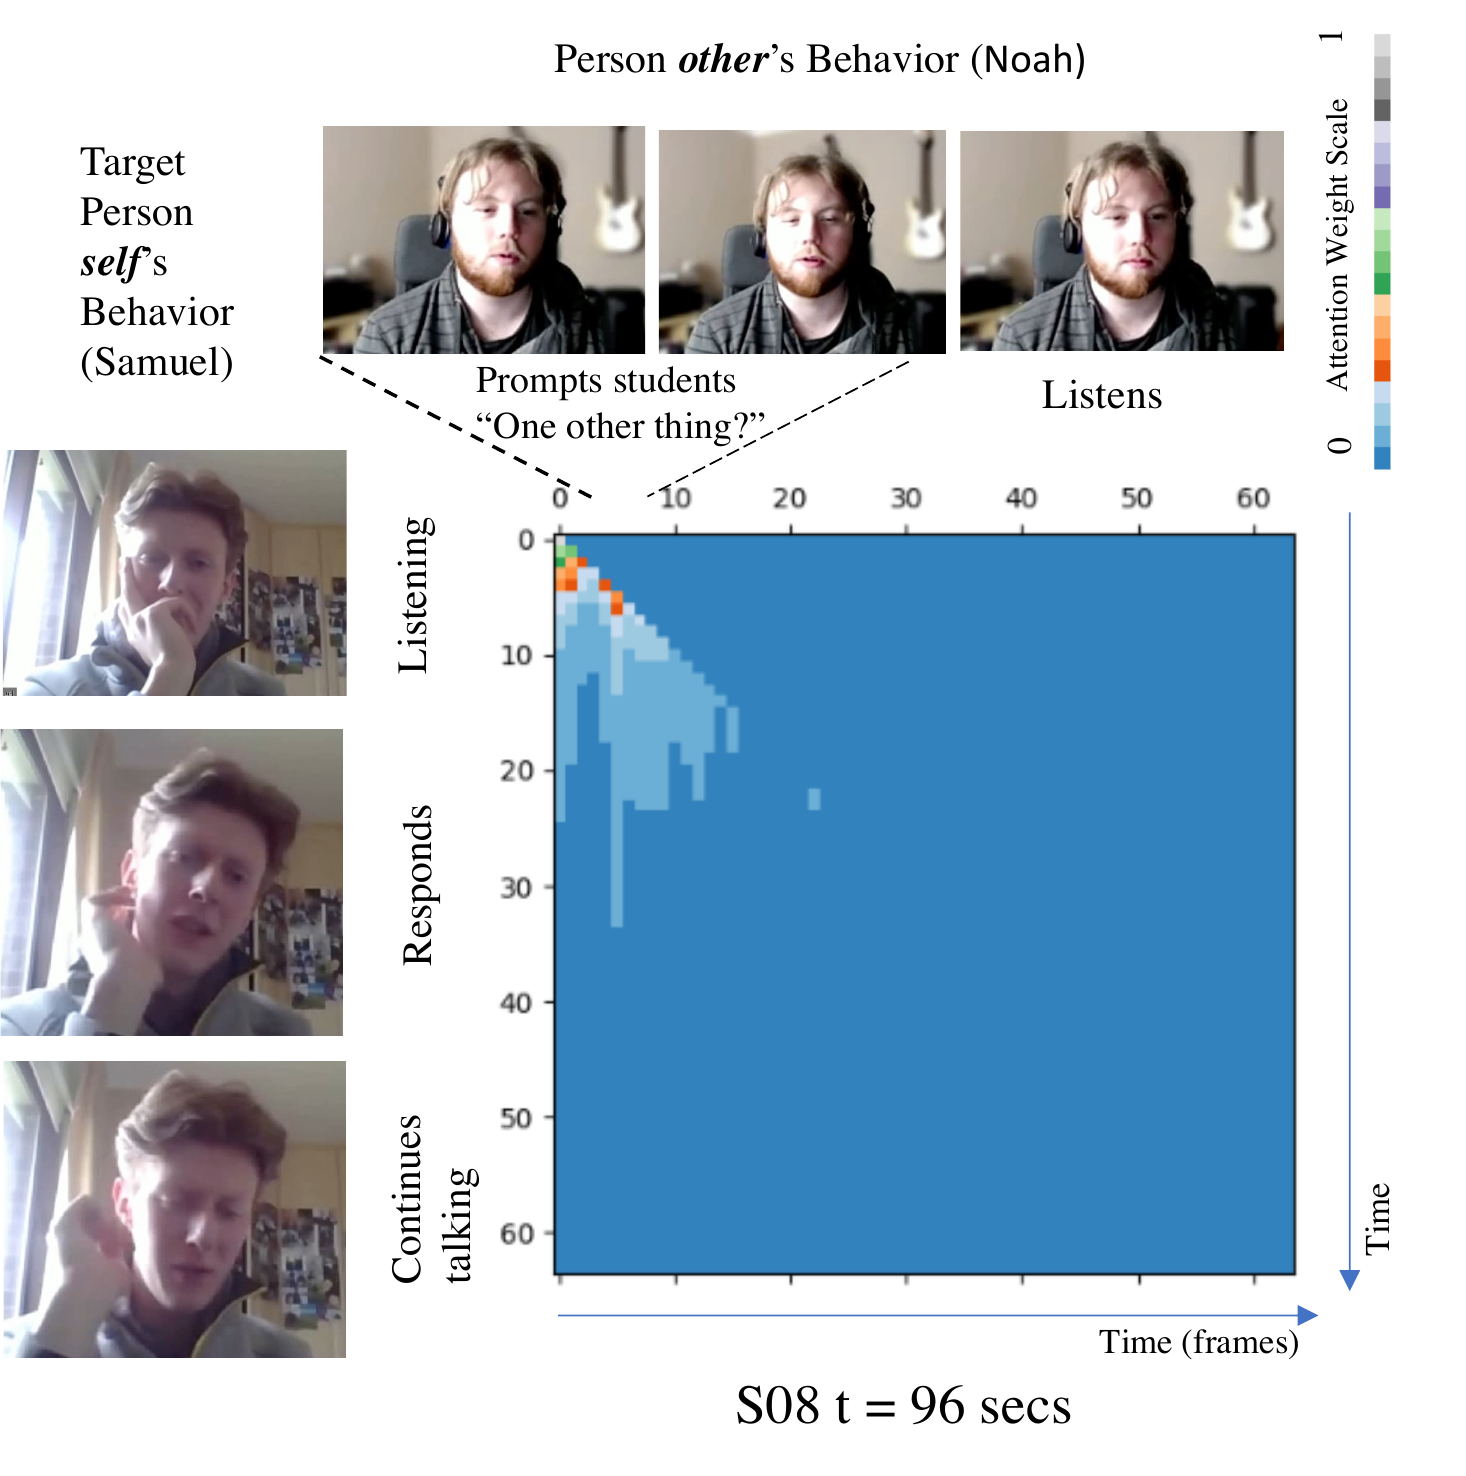}
    \caption{(a) \modelss Cross-person Attention weights from $t=96s$ for group $S08$. \modelshorts has discovered that $self$’s behavior from timestep 10-35 is contingent on $other$’s behavior in timestep 4-7. }

\end{figure*}

\newpage
\section{Additional Attention Weights}
\begin{figure*}[!ht]
    \centering
    \includegraphics[width=0.9\textwidth]{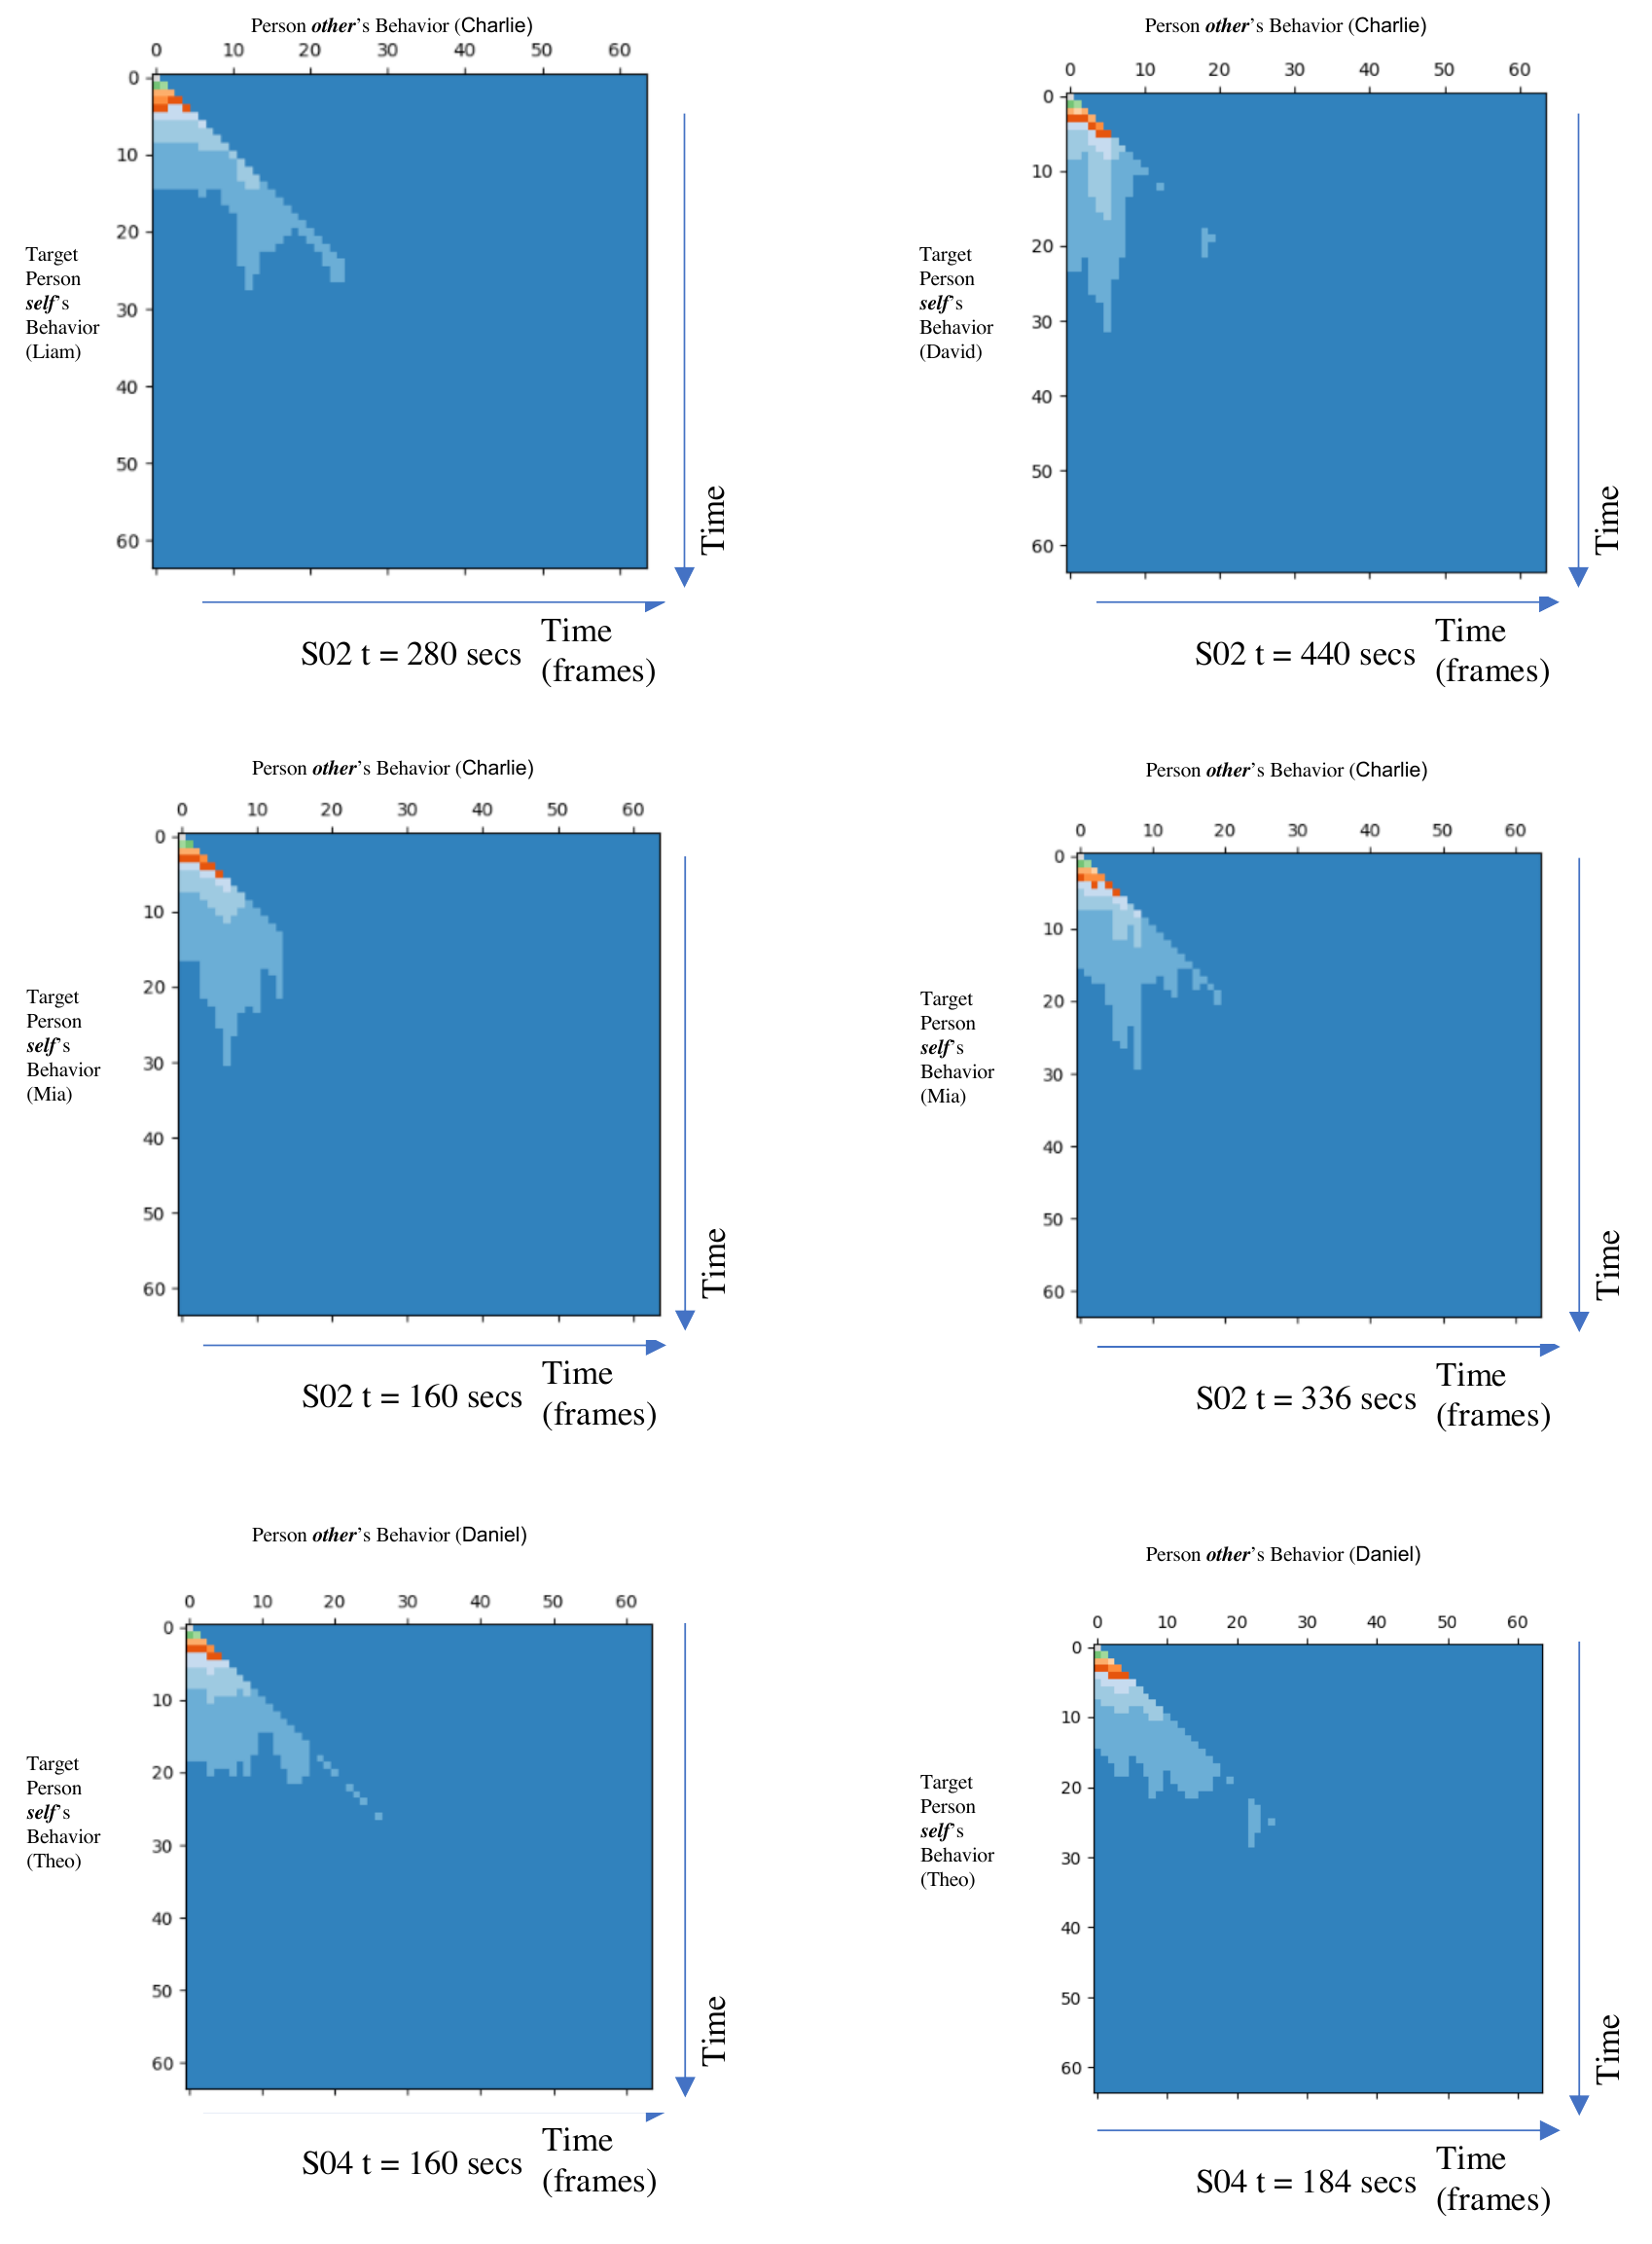}

\end{figure*}

\begin{figure*}[!ht]
    \centering
    \includegraphics[width=0.9\textwidth]{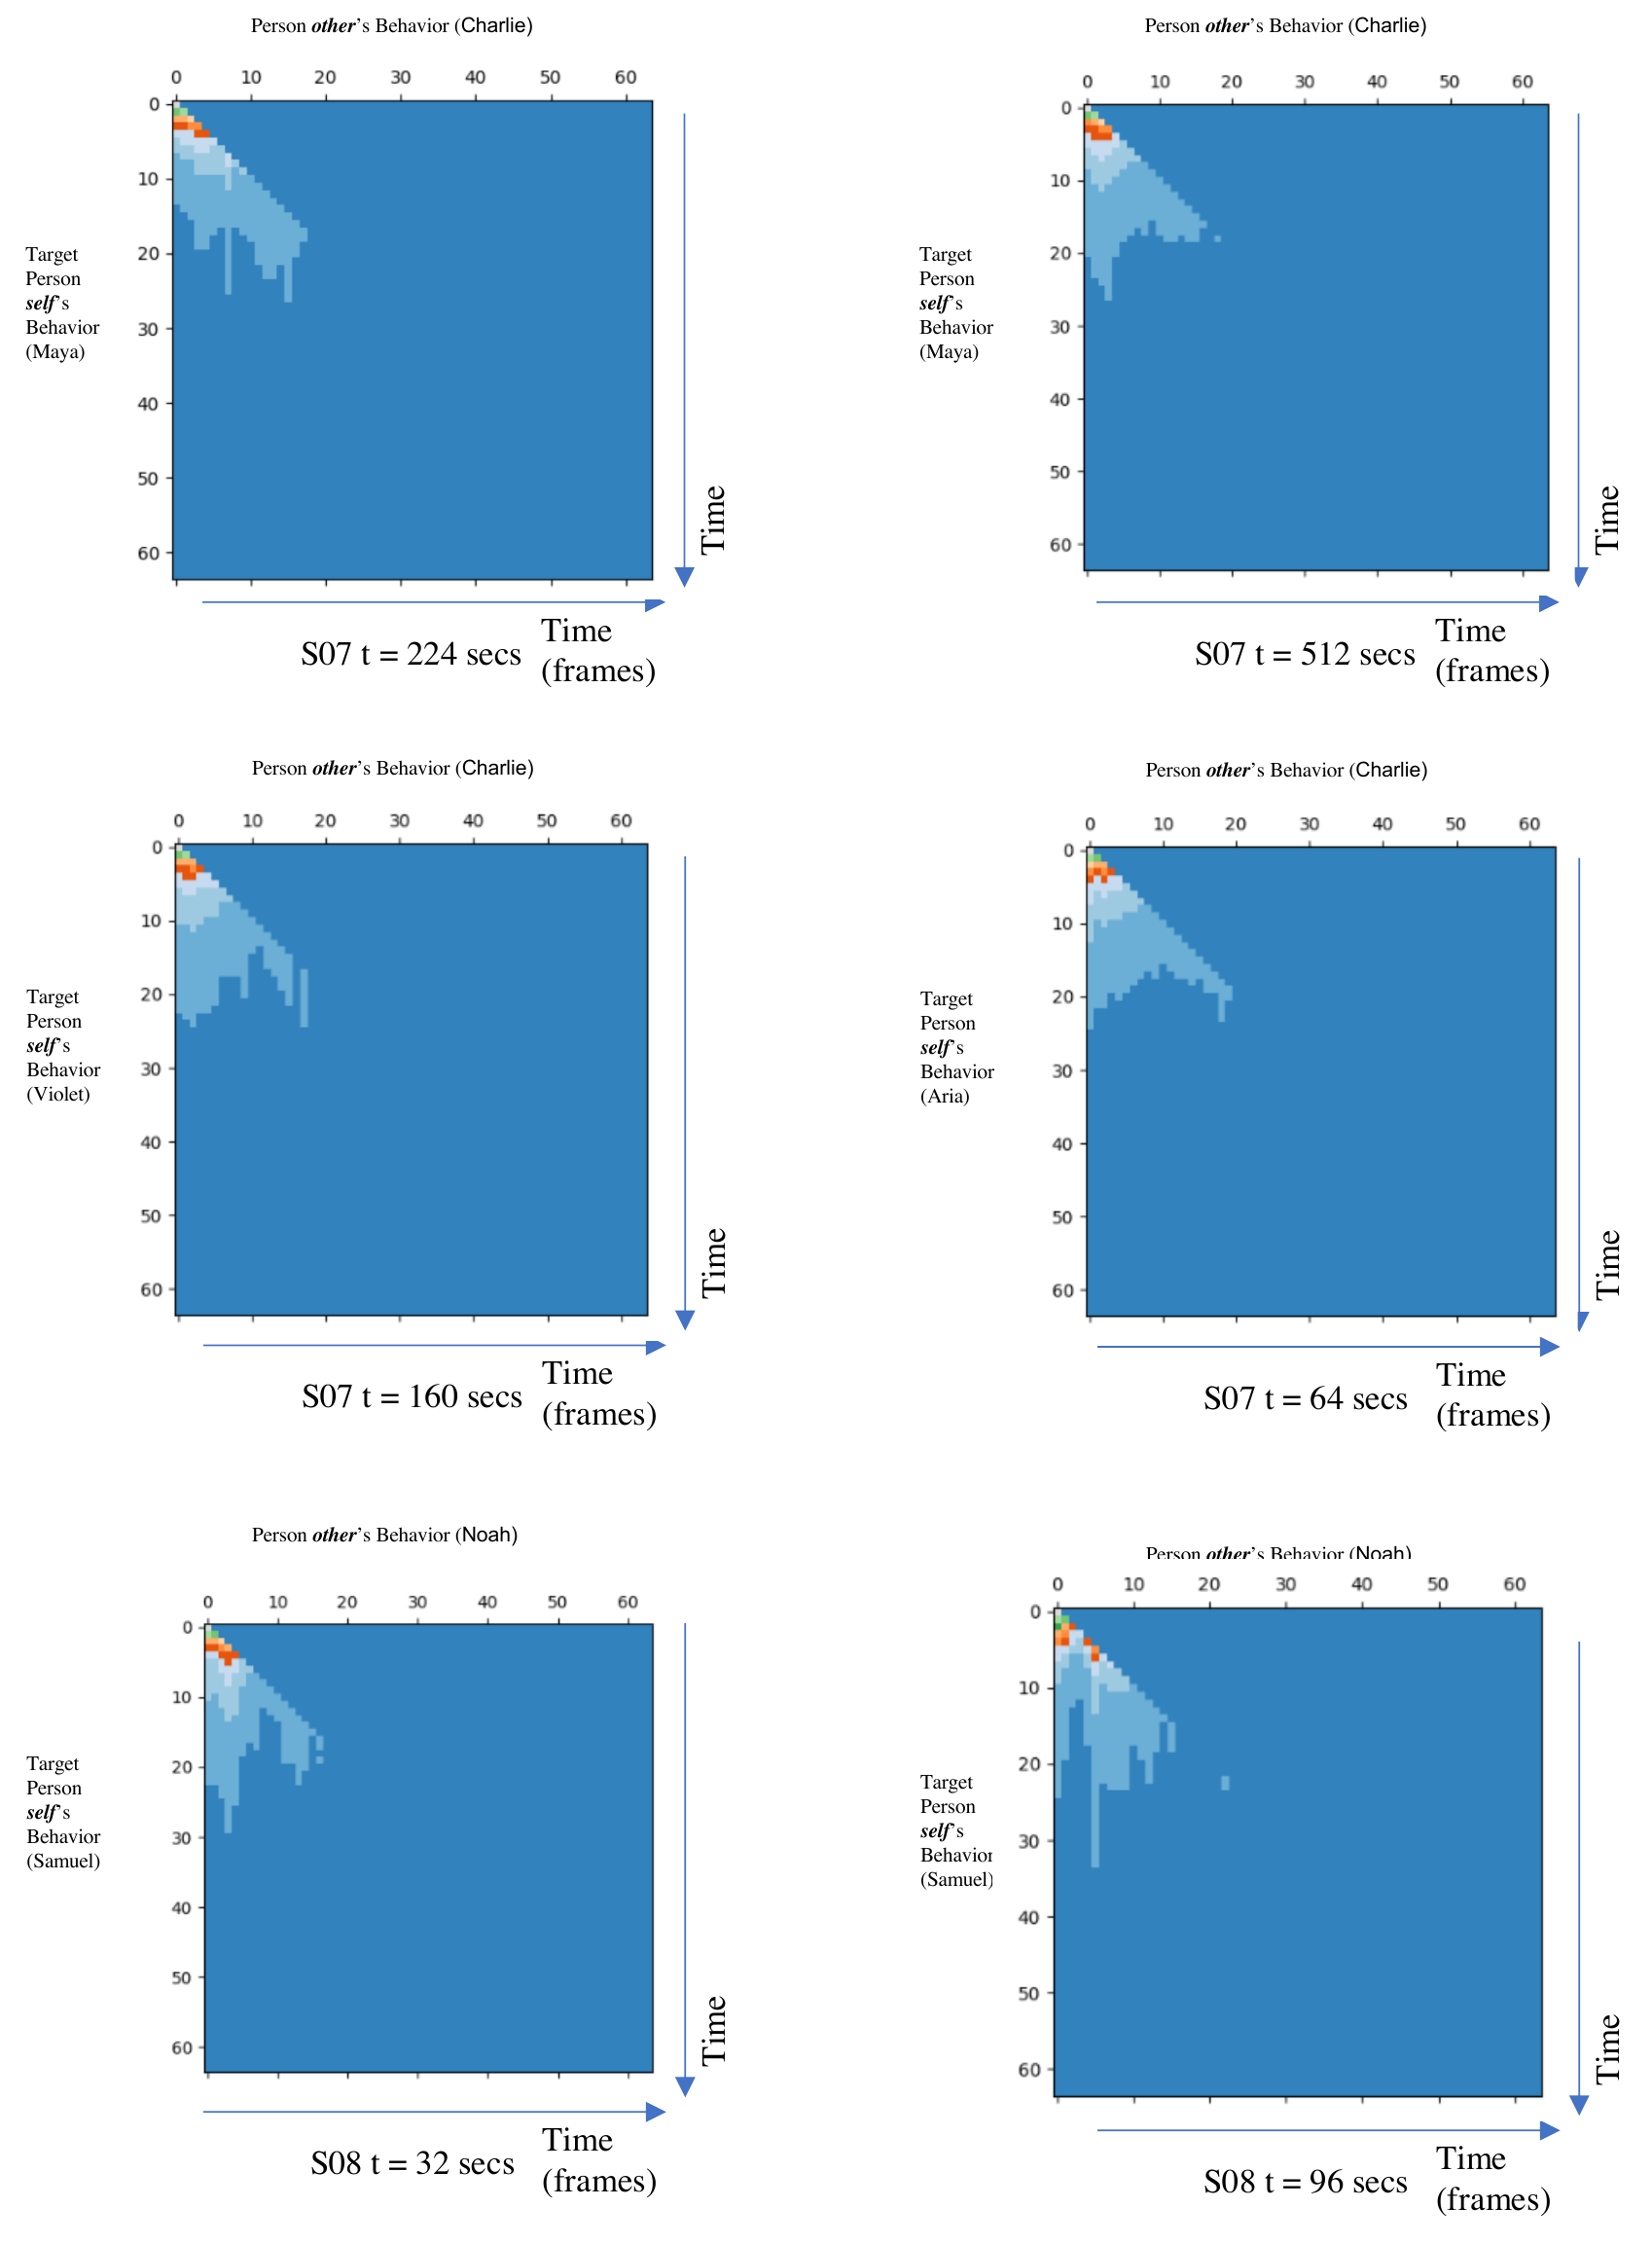}

\end{figure*}

\begin{figure*}[!ht]
    \centering
    \includegraphics[width=0.9\textwidth]{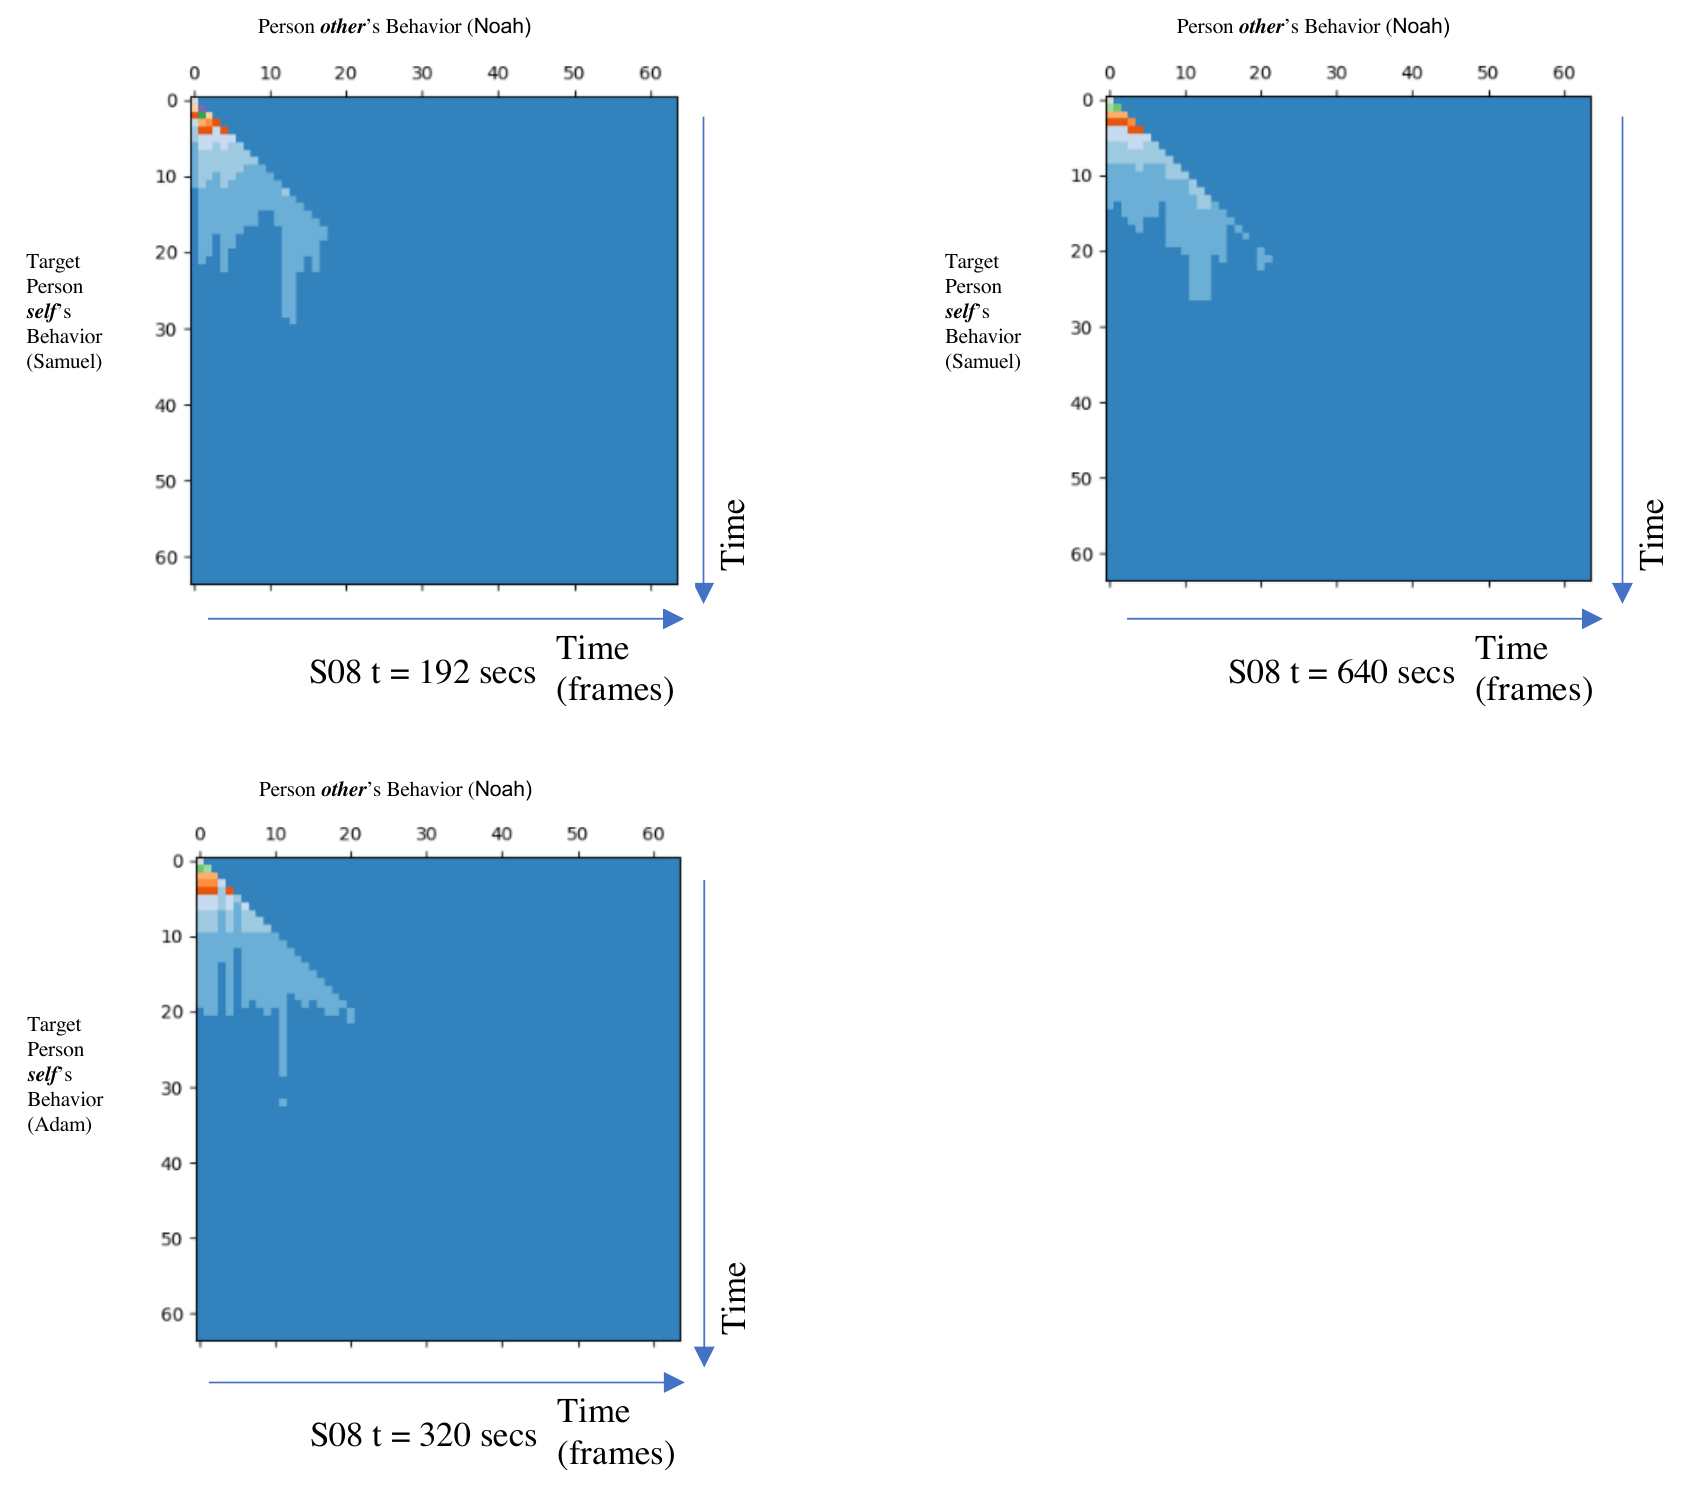}
    \caption{Diverse \modelss Cross-person Attention weights, we see that our model captures non-uniform and interesting attention weights to capture behavior interactions across pairs of people.}

\end{figure*}

\clearpage
\section{Detailed Description of All Baselines}
\label{aref:baselines}

\subsection{Engagement Models:} 
\textbf{ConvLSTM \cite{del2020you}} utilizes a sequence of video frames as input. The frames are processed to intermediate features from a pre-trained ResNetXt-50 Convolutional Neural Network (CNN)(from the activation of the last fully connected layer of the CNN) as inputs to a recurrent LSTM   module. The output of the LSTM is passed through a fully-connected layer to predict engagement values. \textbf{OCtCNN-LSTM \cite{steinert2020towards}} processed each frame of the video as skeletal key points and facial action units from  Openface [CITE] and pre-trained CNN features (VGGFace [CITE]). The two features are fused via concatenation and fed into a multilayered LSTM [CITE]  for prediction.
\textbf{GAT \cite{zhang2022engagement}} the self-attention mechanism is applied to contextualize the behavioral, affective, and visual features. ResNet-3D, DMUE, and OpenFace  are used for each feature extraction. The concatenation of these learned three components gives the representation of an individual, which is then further improved via graph neural networks (GNNs). A graph representation of the group is learned, where a hidden representation of each node in the graph is learned by attending to the rest. In detail, a two-layer graph attention network (GAT) \cite{velivckovic2017graph} is adopted to learn the underlying interactions between nodes by computing attention weights for each edge. The resulting embeddings are fed into fully connected layers which regress to the engagement state. More recently, models that use bootstrapping and ensembling are proposed in \textbf{BOOT \cite{wang2019bootstrap}} and \textbf{ENS-MODEL \cite{thong2019engagement}}. \textbf{HTMIL \cite{ma2021hierarchical}} uses a Bi-LSTM with multi-scale attention and clip-level and video-level objectives, and \textbf{TEMMA \cite{chen2020transformer}} utilizes a Resnet-Transfomer model. Unlike our work, previously proposed approaches do not take into account the group setting; they focus on modeling individuals.

\subsection{Action Recognition Models:} 

\textbf{TimeSformer \cite{bertasius2021spacetime}} a convolution-free video classification model was built exclusively on self-attention over space and time. The model adapts the standard Transformer \cite{DBLP:journals/corr/VaswaniSPUJGKP17} architecture to video by enabling spatiotemporal feature learning directly from a sequence of frame-level patches. 
\textbf{SlowFast \cite{feichtenhofer2019slowfast}} the model involves 1) a slow pathway, operating at a low frame rate, to capture spatial semantics, and 2) a fast pathway, operating at a high frame rate, to capture motion at fine temporal resolution.  
\textbf{I3D \cite{NonLocal2018}} a two-stream inflated 3D ConvNet based on 2D ConvNet inflation is used: filters and pooling kernels of deep image classification ConvNets are expanded into 3D, which enables it to learn seamless spatio-temporal feature extractors from video while utilizing ImageNet architecture designs and their parameters.  

\section{Subjectivity of Engagement}

As mentioned in Section \ref{sec:related}, engagement is a multi-dimensional construct that can be measured in various ways. Furthermore, the target towards which a person is engaged is crucial. In our work, we study on-task, off-task engagement as defined by the RoomReader \cite{reverdy2022roomreader} dataset. Future work should delve into different types of engagement, as they could require different types of reasoning or inductive biases.
